# Supplementary material for: MAMDR: A Model Agnostic Learning Method for Multi-Domain Recommendation
Source: arXiv:2202.12524 source file (2023-03-07)
Supplement: Supplementary file 1 [file appendix.tex]

\section{Appendix}
% In the appendix, we will first give more details of datasets. Following, we will introduce the compared methods, implementation details, and experiment settings used in sections \ref{sec:performance} and \ref{sec:method}. Last, we will present the detailed experimental results of Parameters Analysis to help better understand the performance of our methods.
\subsection{Detailed Related work}
\subsubsection{Multi-Domain Recommendation}
Recommender system has been a long-standing research topic. Recently, many deep learning-based recommender systems have been proposed (e.g., WDL \cite{cheng2016wide}, NeurFM \cite{he2017neural}, and AutoInt \cite{song2019autoint}). However, most of them are designed for single domain recommendation. In the real-world, huge data are collected from multi-domains. Related to MDR, cross-domain recommendation (CDR) aims to improve the performance of the target domain with the help of auxiliary domains \cite{khan2017cross}. CDCF \cite{loni2014cross} extended the traditional matrix factorization to CDR with interacting information from auxiliary domains to target domains. Following the idea of transfer learning, CoNet \cite{hu2018conet} enabled a dual knowledge transfer across domains by introducing cross-connections from two networks. $s^2$Meta \cite{du2019sequential} unified the meta-learning and CDR and learned generic initial parameters for different domains.
In contrast to CDR, our multi-domain recommendation (MDR) problem aims to improve the results of all domains.

The MDR problem has recently garnered considerable attention. MCF \cite{zhang2010multi} applied several collaborative filtering tasks in various domains at the same time to investigate domain connections. Similarly, ICAN \cite{xie2020internal} also focused on the interactions across domains. Ma et al. \cite{ma2018your} enabled the cross-media content features to be used in multi-domain collaborative filtering. Furthermore, AFT \cite{hao2021adversarial} proposed a novel adversarial feature translation to learn features translation between different domains. 
Additionally, by considering each domain as a task, multi-task approaches (e.g., Shared-Bottom \cite{ruder2017overview}) could be simply deployed to tackle the MDR problem. MMoE \cite{ma2018modeling} extended the Shared-Bottom by designing several domain expert networks and a novel multi-gate strategy. On the top of MMoE, PLE \cite{tang2020progressive} proposed a shared-specific expert network to progressively extract specific and multi-domain features. Inspired by MTL, STAR \cite{sheng2021one} separated the model parameters into shared and domain-specific parts. Meanwhile, STAR proposed a novel partitioned normalization to model the distinct distribution of different domains. However, these methods still suffer from the domain conflict and overfitting problems as discussed in the section \ref{sec:introduction}.

\subsubsection{Multi-Domain Learning}

Multi-Domain Learning (MDL) \cite{yang2015unified} has been widely applied in the real-world. Some MDL research can be extended to solve the problems in MDR. 
The domain generalization (DG) methods seek to distill the common knowledge from multi-domains and learn more robust features that are potentially useful for unseen domains. Existing research \cite{li2017deeper} assumed that any domain can be factorized into a shared and domain-specific component. Mansilla et al. \cite{mansilla2021domain} analyzed the multi-domain gradient conflict and adapted the PCGrad \cite{yu2020gradient} into the multi-domain setting. The PCGrad alleviates the gradient conflict of two domains by projecting their gradients into the non-conflict direction. However, this strategy is inefficient for scenarios with more than two domains. MLDG \cite{li2018learning} improved the generalizability of learned parameters by extending the idea of meta-learning. By using meta-learning, Dou et al. \cite{dou2019domain} introduced two complementary losses to explicitly regularize the semantic structure of the feature space.  Similarity, Sicilia et al. \cite{sicilia2021multi} adopted meta-learning to balance the losses between different domains. MetaReg \cite{balaji2018metareg} also adopted the meta-learning as a regularization term to achieve good multi-domain generalization.

\subsubsection{Meta-Learning}

Meta-learning (e.g., MAML \cite{finn2017model} and Reptile \cite{nichol2018first}) aims to learn generalized initialized weights that can be readily tailored to new tasks, which is agnostic to model structure. Meta-learning acquires the shared knowledge across tasks and enables specific information through a few-step finetuning \cite{sun2019meta}. Meta-learning may be used to the MDR problem by treating each task as a domain. To address the gradient conflict, \textcolor{blue}{MT-net \cite{lee2018gradient} enables the parameters to be learned on task-specific subspaces with distinct gradient descent. WarpGrad \cite{flennerhag2019meta} further proposed a Warped Gradient Descent that facilitates the gradient descent across the task distribution. L2F \cite{baik2020learning} introduced a task-and-layer-wise attenuation mask on the initial parameters to alleviate the conflict among tasks. GradDrop \cite{tseng2020regularizing} presented a meta-learning-based Gradient Dropout to avoid overfitting for certain tasks. TADAM \cite{oreshkin2018tadam} developed a metric scaling method to provide task-dependent metric space for optimizing specific parameters. HSML \cite{yao2019hierarchically} introduced a hierarchical task clustering structure to preserve generalization knowledge among tasks, while also maintaining the specific information.}

Even some multi-domain learning and meta-learning frameworks can be applied to the MDR problem, they are not as effective as the proposed \ourmethod. Our method enables scalable implementation in the large-scale MDR problem and is compatible with the existing recommendation models.

\subsection{Large-scale Implementation}\label
{sec:implementation}
In this section, we will introduce the implementation of MAMDR in our large-scale application setting.
To support large-scale applications, we adopt the PS-Worker architecture \cite{li2014scaling} for distributed training. PS-Worker is a commonly used data-parallel method for scaling model training on multiple machines, which contains two parts of machine: parameter servers and workers. Parameter servers store model parameters, and workers calculate the gradients.

The overall architecture is illustrated in Figure \ref{fig:psworker}. (1) we first distribute the training data into $m$ worker machines. (2) each worker obtains the parameters from the parameter server and stores as the local parameter. (3) the \ourmethod algorithm is implemented in each worker to update the local parameters and compute the local gradient. (4) workers send their local gradients to the parameter server. (5) the parameter server synthesizes the local gradients and updates the model parameters. In this way, we can implement \ourmethod in our applications to deal with billions of data.
\begin{figure}[t]
    \centering
    \includegraphics[trim=0cm 0cm 0cm 0,clip,width=0.5\columnwidth]{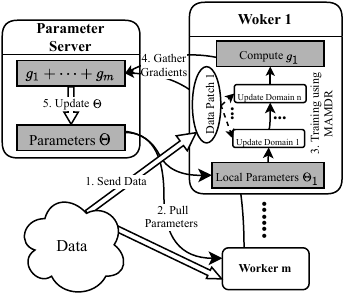}
    \caption{Implementation of \ourmethod in PS-Worker architecture.}
    \label{fig:psworker}
\end{figure}

\subsection{Datasets}\label{app:datasets}
In this section, we will detail the dataset used in our experiment. The statistic of datasets is given in Table \ref{tab:dataset}.
The public datasets used in our experiments can be found at: Amazon\footnote{\url{https://nijianmo.github.io/amazon/index.html}} and Taobao\footnote{\url{https://tianchi.aliyun.com/dataset/dataDetail?dataId=649}}. Amazon dataset originally contains 29 categories of products, such as ``Musical Instruments'' and ``Video Games''. \textcolor{red}{Due to the limitation of GPU memory, we cannot handle the complete dataset. Therefore, for Amazon, we first select 6 domains with relatively abundant interactions as Amazon-6. Then, we select 7 more domains with fewer interactions to simulate the data sparsity situation and construct Amazon-13, where the overfitting is more likely to occur.} As the Amazon dataset does not provide negative samples, we randomly select products not rated by a specific user as negative samples. The number of negative samples is selected by the given CTR Ratio of each domain.
The CTR ratio is defined as:
\begin{equation}
    \setlength\abovedisplayskip{1pt}%shrink space
    \setlength\belowdisplayskip{1pt}
    \text{CTR Ratio} = \frac{\text{\# positive samples}}{\text{\# negative samples}}.
\end{equation}
We randomly assign CTR Ratio for each domain, ranging from $[0.2,0.5]$, to simulate the domain distinction. For Amazon-6 and Amazon-13, the category, sample number, sample percentage, and CTR Ratio of each domain are listed in Table \ref{tab:amazon6} and Table \ref{tab:amazon13}.

Taobao dataset contains users' click logs from different themes of purchase, e.g.,``what to take when traveling'', ``how to dress up yourself for a party'', and ``things to prepare when a baby is coming''. \textcolor{red}{We treat each theme as a domain and try to increase the number of domains as large as possible. Despite more domains introducing more training samples could improve the overall performance, but this would also increase the probability of domain conflict. Thus, we respectively select 10/20/30 themes to construct Taobao-10/20/30.} Similarly, the CTR Ratio is randomly selected from  $[0.2,0.5]$. The statistics of the selected 30 domains are listed in Table \ref{tab:taobao}. The first 10 and 20 domains are used for Taobao-10 and Taobao-20, respectively.

The industry dataset is collected from our online shopping application, which cannot be public due to the privacy issue. This dataset contains 69,102 different domains and 489,852,853 samples. The details of industry dataset dataset are shown in Table \ref{tab:taobaoonline}. From the statistic, we can see that the industry dataset has more domains but a smaller CTR Ratio than public datasets, which is more challenging for the existing models.
\begin{table}[htbp]
    \centering
    %\Huge
    \caption{Overall statistic of datasets.}
    \label{tab:dataset}
    \resizebox{1\columnwidth}{!}{%
        \begin{tabular}{cccccccc}
            \toprule
            Dataset   & \# Domain & \# User    & \# Item    & \# Train    & \# Val     & \# Test    & Sample / Domain \\
            \midrule
            Amazon-6  & 6         & 445,789    & 172,653    & 9,968,333   & 3,372,666  & 3,585,877  & 2,821,146       \\
            Amazon-13 & 13        & 502,222    & 215,403    & 11,999,607  & 4,100,756  & 4,339,523  & 1,572,299       \\\midrule
            Taobao-10 & 10        & 23,778     & 6,932      & 92,137      & 37,645     & 43,502     & 17,328          \\
            Taobao-20 & 20        & 58,190     & 16,319     & 243,592     & 96,591     & 106,500    & 22,334          \\
            Taobao-30 & 30        & 99,143     & 29,945     & 394,805     & 151,369    & 179,252    & 24,180          \\\midrule
            Industry  & 69,102    & 84,307,785 & 16,385,662 & 420,097,203 & 23,340,352 & 46,415,298 & 7,088           \\
            \bottomrule
        \end{tabular}
    }
\end{table}
\begin{table*}[]
    \centering
    \begin{minipage}{1\linewidth}
        \centering
        \Huge
        \caption{Statistics of Amazon-6 dataset.}
        \label{tab:amazon6}
        \resizebox{1\linewidth}{!}{%
            \begin{tabular}{@{}ccccccc@{}}
                \toprule
                Domain     & Musical Instruments & Office Products & Patio Lawn and Garden & Prime Pantry & Toys and Games & Video Games \\ \midrule
                \# Samples & 1204340             & 3921259         & 3025218               & 694758       & 5382501        & 2698800     \\
                Percentage & 7.11\%              & 23.17\%         & 17.87\%               & 4.10\%       & 31.80\%        & 15.94\%     \\
                CTR Ratio  & 0.22                & 0.23            & 0.32                  & 0.23         & 0.47           & 0.21        \\ \bottomrule
            \end{tabular}
        }
    \end{minipage}
    \begin{minipage}{1\linewidth}
        \centering
        \Huge
        \centering
        \Huge
        \caption{Statistics of Amazon-13 dataset.}
        \label{tab:amazon13}
        \resizebox{\linewidth}{!}{%
            \begin{tabular}{@{}cccccccccccccc@{}}
                \toprule
                Domain     & Arts Crafts and Sewing & Digital Music & Gift Cards & Industrial and Scientific & Luxury Beauty & Magazine Subscriptions & Musical Instruments & Office Products & Patio Lawn and Garden & Prime Pantry & Software & Toys and Games & Video Games \\ \midrule
                \# Samples & 2419005                & 770132        & 11951      & 380386                    & 87360         & 13103                  & 814928              & 3178096         & 2317603               & 655970       & 11022    & 7541261        & 459646      \\
                Percentage & 12.96\%                & 4.13\%        & 0.06\%     & 2.04\%                    & 0.47\%        & 0.07\%                 & 4.37\%              & 17.03\%         & 12.42\%               & 3.52\%       & 0.06\%   & 40.41\%        & 2.46\%      \\
                CTR Ratio  & 0.22                   & 0.23          & 0.32       & 0.23                      & 0.47          & 0.21                   & 0.36                & 0.30            & 0.46                  & 0.25         & 0.30     & 0.30           & 0.27        \\ \bottomrule
            \end{tabular}
        }
    \end{minipage}
    \begin{minipage}{1\linewidth}
        \centering
        \Huge
        \caption{Statistics of Taobao-10/20/30 dataset.}
        \label{tab:taobao}
        \resizebox{\linewidth}{!}{%
            \begin{tabular}{@{}ccccccccccccccccccccccccccccccc@{}}
                \toprule
                Domain     & D1     & D2     & D3     & D4     & D5     & D6     & D7     & D8     & D9     & D10    & D11    & D12    & D13    & D14     & D15    & D16    & D17    & D18    & D19    & D20    & D21    & D22    & D23    & D24    & D25    & D26    & D27    & D28    & D29    & D30    \\ \midrule
                \# Sample  & 13255  & 7007   & 20130  & 62460  & 11563  & 7190   & 4185   & 24052  & 5582   & 17860  & 29302  & 6472   & 8873   & 125586  & 15560  & 5458   & 14095  & 53910  & 12102  & 2936   & 4710   & 29256  & 41609  & 7354   & 68119  & 5308   & 24918  & 38919  & 24297  & 34253  \\
                Percentage & 1.82\% & 0.96\% & 2.77\% & 8.60\% & 1.59\% & 0.99\% & 0.58\% & 3.31\% & 0.77\% & 2.46\% & 4.03\% & 0.89\% & 1.22\% & 17.29\% & 2.14\% & 0.75\% & 1.94\% & 7.42\% & 1.67\% & 0.40\% & 0.65\% & 4.03\% & 5.73\% & 1.01\% & 9.38\% & 0.73\% & 3.43\% & 5.36\% & 3.35\% & 4.72\% \\
                CTR Ratio  & 0.22   & 0.23   & 0.32   & 0.23   & 0.47   & 0.21   & 0.36   & 0.30   & 0.46   & 0.25   & 0.30   & 0.30   & 0.27   & 0.20    & 0.33   & 0.23   & 0.38   & 0.22   & 0.29   & 0.33   & 0.47   & 0.23   & 0.24   & 0.44   & 0.21   & 0.47   & 0.37   & 0.28   & 0.45   & 0.43   \\ \bottomrule
            \end{tabular}
        }
    \end{minipage}
    \begin{minipage}{1\linewidth}
        \centering
        \caption{Statistics of industry dataset.}
        \label{tab:taobaoonline}
        \resizebox{\linewidth}{!}{%
            \begin{tabular}{@{}cccccccccc@{}}
                \toprule
                Dataset  & \# Sample   & \# User    & \# Item    & \# Domain & \# Train    & \# Val     & \# Test    & Sample / Domain & CTR Ratio \\ \midrule
                Industry & 489,852,853 & 84,307,785 & 16,385,662 & 69,102    & 420,097,203 & 23,340,352 & 46,415,298 & 7,088           & 0.0474    \\ \bottomrule
            \end{tabular}
        }
    \end{minipage}
\end{table*}

\subsection{Experiment settings of Performance Comparison}\label{app:performance}

In this section, we will detail the baselines and experiment settings used in performance comparison.

\subsubsection{Baselines}
We select several state-of-the-art methods in CTR prediction as baselines, which can be roughly grouped into two categories: Single-Domain method and Multi-Task (Domain) method.

\textbf{Single-Domain Method.} This group of methods is originally proposed for single domain recommendation. Thus, they do not consider the domain distinction information.
\begin{itemize}
    \item MLP: Multi-layer perceptron (MLP) is the simplest neural network model composed of multiple fully connected layers.
    \item WDL \cite{cheng2016wide}: WDL is a widely used recommendation model in the industry. It contains a wide liner network and a deep neural network to simultaneously capture the cross-product features as well as the nonlinear features.
    \item NeurFM \cite{he2017neural}: NeurFM proposes a bi-interaction pooling layer to learn feature interaction between embedding vectors. Then, it integrates the results with the logit output of a MLP layer.
    \item AutoInt \cite{song2019autoint}: AutoInt proposes the attention-based interaction layer to automatically identify meaningful high-order features.
    \item DeepFM \cite{guo2017deepfm} integrate the factorization machine with the deep neural network to improve the recommendation results.
\end{itemize}

\textbf{Multi-Task (Domain) Method.} This group of methods contains the multi-task and multi-domain methods. As discussed in the Introduction, the multi-task methods can be directly applied to MDR by treating each domain as a separate task.
\begin{itemize}
    \item Shared-Bottom \cite{ruder2017overview}: Shared-Bottom is a multi-task method that consists of shared-bottom networks and several domain-specific tower networks. Each domain has its specific tower network while sharing the same bottom network.
    \item MMOE \cite{ma2018modeling}: MMOE adopts the  Mixture-of-Experts (MoE) structure by sharing the expert modules across all domains, while having a gating network trained for each domain.
    \item PLE \cite{tang2020progressive}: PLE separates shared components and task-specific components explicitly and adopts a progressive mechanism to extract features gradually.
    \item Star \cite{sheng2021one} is the state-of-the-art MDR method. It splits the parameters into shared and specific parts. Meanwhile, it proposes a Partitioned Normalization for distinct domain statistics.
\end{itemize}

\subsubsection{Implementation Details}\label{app:parameters}
All the models in single-domain and multi-domain methods, except the Star, are implemented by DeepCTR \cite{shen2017deepctr}, which is an open-source deep-learning based CTR package. Star is implemented by us according to the original paper.

To make a fair comparison, we try to set similar parameters for all the models. For all single-domain methods, the hidden layers are set to $[256,128,64]$; for AutoInt, its attention head number is set to $4$; for Shared-bottom, its shared network is set to $[512,256,128]$ and its tower network is set to $[64]$; for MMOE, its expert networks are set to $[512,256,128]$, its tower network and gating network are set to $[64]$, and its expert number is set to $2$; for PLE, its shared network is set to $[64]$, its tower network is set to $[256]$, its gating network is set to $[64]$, its shared and specific experts are set to $2$ and $10$, respectively, and the progressive level is set to $1$; for Star, both the shared and specific networks are set as $[256,128,64]$. For all models, the dropout rate are set to 0.5, the embedding size is set to 128, and the learning rate is set to 0.001. For our \ourmethod, the inner learning rate is set to 0.001, and the outer learning rate is set to 0.1; the sample number of DR is set to $[3,5,5,5,5]$ for each dataset respectively. We use Adam as the optimizer and Binary Cross Entropy as the recommendation loss function. Experiments are conducted on a RTX2080 GPU with 64G RAM.

\subsection{Experiment Settings of Learning Framework Comparison}\label{app:methods}
In this section, we detail the learning frameworks used in learning framework comparison, which can be roughly grouped into three categories: traditional learning frameworks, multi-task leaning method, and meta-learning frameworks.

\textbf{Traditional Learning Frameworks.}
\begin{itemize}
    \item Alternate: Alternate learning is a conventional learning framework that trains on multiple domains alternately. In this way, it enables the model to learn shared features and improve performance.
    \item Alternate + Finetune: On the top of the model learned by Alternate learning, we finetune the model on each domain to obtain several domain-specific models. Each specific model can capture the domain distinction information.
\end{itemize}

\textbf{Multi-Task Learning Frameworks.}
\begin{itemize}
    \item Weighted Loss \cite{kendall2018multi}: Weighted Loss is a multi-task learning framework that assigns weight to the loss of each task. Meanwhile, the weight is automatically optimized during the training to balance between different losses.
    \item PCGrad \cite{yu2020gradient}: PCGrad is a powerful multi-task learning framework. By projecting the gradients of each task into the normal plane of others, it successfully avoids the conflicting problem.
\end{itemize}

\textbf{Meta-Learning Frameworks.}
\begin{itemize}
    \item MAML \cite{finn2017model}: MAML aims to train parameters through various tasks and acquires parameters that can quickly adapt to new tasks. We treat each domain as the task and split the training data into the support and query sets used for MAML.
    \item Reptile \cite{nichol2018first}: Reptile is a first-order meta-learning framework, which trains parameters by rapidly sampling the tasks. It maximizes the inner-gradients within the task and leads parameters quickly to generalize to new tasks.
    \item MLDG \cite{li2018learning}: MLDG proposes a novel meta-learning framework for domain generalization. Its meta-optimization function improves the performance on both train and test domains.
\end{itemize}

We implement all the learning frameworks in Tensorflow and conduct experiments on the Taobao-10 dataset.

\subsection{Experiment Settings of industry application}\label{app:methods}
In industry dataset, we adopt the distributed training framework illustrated in Figure \ref{fig:psworker}. The baseline models are trained in Alternate Training by default. We also compare our \ourmethod with the Separate Training method, which optimizes a separate model for each domain.

\subsection{Detailed Experiment Results of Each Domain}\label{app:detailed}
\textcolor{red}{To better understand the results of each domain, we will show the detailed results of each domain in Table \ref{tab:amazon-6-specific}, \ref{tab:amazon-13-specific},\ref{tab:taobao-10-specific}, \ref{tab:taobao-20-specific}, and \ref{tab:taobao-30-specific}.
From results, we can see that MAMDR reaches the best performance in most domains. Multi-task/domain methods (e.g., Shared-bottom and MMOE) have the second best result. Specifically, for the data richness domain (e.g., "Toys and Games"), single domain methods can reach a good performance, but they perform worse in the data sparsity domain. For example, the "Gift Cards" and "Software" domains have only 11,951 and 11,022 samples. Thus, many single domain methods (e.g., MLP) are overfitting in these domains, whereas DR enables the model to learn from other domains and successfully alleviates the overfitting and greatly improves the performance. Multi-task/domain methods use shared parameters to transfer knowledge for sparsity domains, which suffer the domain conflict problem. Our DN relieves the conflict and improve the performance. Besides, DN can also be applied to existing multi-task/domain methods to improve their performances.}

\begin{table}[h]
    \caption{Results of each domain on Amazon-6 dataset.}
    \label{tab:amazon-6-specific}
    \resizebox{\textwidth}{!}{%
        \begin{tabular}{@{}cccccccc@{}}
            \toprule
            \textbf{Method} & \textbf{Avg.}   & \textbf{Musical Instruments} & \textbf{Office Products} & \textbf{Patio Lawn and Garden} & \textbf{Prime Pantry} & \textbf{Toys and Games} & \textbf{Video Games} \\ \midrule
            MLP             & 0.7464          & 0.7223                       & 0.7257                   & 0.7509                         & 0.7571                & 0.7423                  & 0.7804               \\
            WDL             & 0.7449          & 0.7641                       & 0.7320                   & 0.7145                         & 0.7553                & 0.7533                  & 0.7500               \\
            NFM             & 0.6152          & 0.7343                       & 0.7843                   & 0.6817                         & 0.5001                & 0.4806                  & 0.5103               \\
            AutoInt         & 0.7531          & 0.7300                       & 0.7716                   & 0.7683                         & 0.7554                & 0.7159                  & 0.7777               \\
            DeepFM          & 0.7532          & 0.7226                       & 0.7397                   & 0.7485                         & 0.6946                & 0.7166                  & 0.7779               \\
            Shared-bottom   & 0.7794          & 0.7733                       & 0.8064                   & 0.7705                         & \textbf{0.7611}       & 0.7672                  & 0.7977               \\
            MMOE            & 0.7816          & 0.7718                       & 0.8049                   & \textbf{0.7713}                & 0.7601                & 0.7718                  & 0.8094               \\
            PLE             & 0.7801          & 0.7660                       & 0.8024                   & 0.7699                         & 0.7593                & 0.7846                  & 0.7984               \\
            Star            & 0.7719          & 0.7645                       & 0.7939                   & 0.7671                         & 0.7533                & 0.7690                  & 0.7833               \\
            MLP+DN          & 0.7678          & 0.7544                       & 0.7840                   & 0.7533                         & 0.7140                & 0.7602                  & 0.7763               \\
            MLP+DR          & 0.7822          & 0.7617                       & 0.7940                   & 0.7583                         & 0.7498                & 0.7918                  & 0.8371               \\
            MLP+MAMDR       & \textbf{0.7957} & \textbf{0.7753}              & \textbf{0.8116}          & 0.7579                         & 0.7579                & \textbf{0.8108}         & \textbf{0.8394}      \\ \bottomrule
        \end{tabular}%
    }
\end{table}
\begin{table}[h]
    \caption{Results of each domain on Amazon-13 dataset.}
    \label{tab:amazon-13-specific}
    \resizebox{\textwidth}{!}{%
        \begin{tabular}{@{}ccccccccccccccc@{}}
            \toprule
            \textbf{Method} & \textbf{Avg.}   & \textbf{Arts Crafts and Sewing} & \textbf{Digital Music} & \textbf{Gift Cards} & \textbf{Industrial and Scientific} & \textbf{Luxury Beauty} & \textbf{Magazine Subscriptions} & \textbf{Musical Instruments} & \textbf{Office Products} & \textbf{Patio Lawn and Garden} & \textbf{Prime Pantry} & \textbf{Software} & \textbf{Toys and Games} & \textbf{Video Games} \\ \midrule
            MLP             & 0.7016          & 0.5006                          & 0.6324                 & 0.4984              & 0.6816                             & 0.7303                 & 0.7126                          & 0.7287                       & 0.7662                   & 0.7585                         & 0.6976                & 0.4989            & 0.6680                  & 0.7809               \\
            WDL             & 0.7026          & 0.5617                          & 0.6561                 & 0.7188              & 0.6517                             & 0.7158                 & 0.7179                          & 0.7368                       & 0.7422                   & 0.7622                         & 0.7458                & 0.6680            & 0.7036                  & 0.7539               \\
            NFM             & 0.6505          & 0.7272                          & 0.4994                 & 0.6628              & 0.5017                             & 0.7123                 & 0.6795                          & 0.7486                       & 0.4991                   & 0.7304                         & 0.7239                & 0.6454            & 0.5655                  & 0.7611               \\
            AutoInt         & 0.7214          & 0.7490                          & 0.6721                 & 0.7308              & 0.6868                             & 0.7792                 & 0.7087                          & 0.7621                       & 0.6766                   & 0.7217                         & 0.7468                & 0.7040            & 0.7430                  & 0.6969               \\
            DeepFM          & 0.6976          & 0.6520                          & 0.6209                 & 0.7041              & 0.6864                             & 0.7423                 & 0.6183                          & 0.7619                       & 0.7448                   & 0.7466                         & 0.6276                & 0.6782            & 0.7107                  & 0.7743               \\
            Shared-bottom   & 0.7088          & 0.7523                          & 0.6504                 & 0.7185              & 0.7011                             & 0.7911                 & \textbf{0.7197}                 & \textbf{0.7713}              & \textbf{0.8008}          & 0.7296                         & 0.7595                & 0.7235            & 0.5005                  & 0.5964               \\
            MMOE            & 0.7381          & 0.7532                          & 0.6731                 & 0.6997              & \textbf{0.7087}                    & 0.7810                 & 0.6809                          & 0.7669                       & 0.7981                   & \textbf{0.7567}                & \textbf{0.7596}       & 0.7216            & 0.7196                  & 0.7766               \\
            PLE             & 0.7114          & 0.7552                          & 0.6116                 & 0.7135              & 0.6590                             & 0.7878                 & 0.7207                          & 0.7326                       & 0.8001                   & 0.7518                         & 0.7044                & 0.7216            & 0.4993                  & 0.7898               \\
            Star            & 0.7209          & 0.7374                          & 0.6639                 & 0.7130              & 0.6905                             & 0.7600                 & 0.6288                          & 0.7595                       & 0.7631                   & 0.7464                         & 0.7314                & 0.6815            & 0.7359                  & 0.7607               \\
            MLP+DN          & 0.7331          & 0.7472                          & 0.6539                 & 0.7248              & 0.6896                             & 0.7370                 & 0.7181                          & 0.7643                       & 0.7879                   & 0.7405                         & 0.7522                & 0.6785            & 0.7602                  & 0.7757               \\
            MLP+DR          & 0.7507          & \textbf{0.7703}                 & 0.6723                 & \textbf{0.7654}     & 0.6716                             & 0.8230                 & 0.6940                          & 0.7468                       & 0.7655                   & 0.7261                         & 0.7381                & 0.7630            & 0.8047                  & 0.8179               \\
            MLP+MAMDR       & \textbf{0.7577} & 0.7454                          & \textbf{0.6853}        & 0.7503              & 0.6725                             & \textbf{0.8325}        & 0.7129                          & 0.7591                       & 0.7964                   & 0.7536                         & 0.7524                & \textbf{0.7553}   & \textbf{0.8129}         & \textbf{0.8212}      \\ \bottomrule
        \end{tabular}%
    }
\end{table}
\begin{table}[h]
    \centering
    \caption{Results of each domain on Taobao-10 dataset.}
    \label{tab:taobao-10-specific}
    \resizebox{\textwidth}{!}{%
        \begin{tabular}{@{}cccccccccccc@{}}
            \toprule
            Method        & Avg.            & 1               & 2               & 3               & 4               & 5               & 6               & 7               & 8               & 9               & 10              \\ \midrule
            MLP           & 0.7022          & 0.6976          & 0.6089          & 0.6760          & 0.7665          & 0.7989          & 0.7347          & 0.6246          & 0.7559          & 0.6684          & 0.6903          \\
            WDL           & 0.7154          & 0.7105          & 0.6292          & 0.6863          & 0.7745          & 0.8089          & 0.7515          & 0.6582          & 0.7691          & 0.6663          & 0.6997          \\
            NFM           & 0.7374          & \textbf{0.7379} & \textbf{0.6573} & 0.6946          & 0.7791          & 0.7961          & \textbf{0.7777} & \textbf{0.6813} & \textbf{0.8285} & 0.6796          & 0.7415          \\
            AutoInt       & 0.7302          & 0.7206          & 0.6421          & 0.6868          & 0.7912          & 0.8065          & 0.7589          & 0.6333          & 0.8239          & 0.6827          & 0.7564          \\
            DeepFM        & 0.7271          & 0.7202          & 0.6411          & 0.6700          & 0.7672          & 0.8076          & 0.7675          & 0.6660          & 0.8310          & 0.6711          & 0.7296          \\
            Shared-bottom & 0.7197          & 0.7081          & 0.6284          & 0.6898          & 0.7969          & 0.8108          & 0.7603          & 0.6367          & 0.7711          & 0.6605          & 0.7343          \\
            MMOE          & 0.7250          & 0.7113          & 0.6383          & 0.6932          & 0.8036          & 0.8135          & 0.7604          & 0.6328          & 0.7777          & 0.6726          & 0.7462          \\
            PLE           & 0.7287          & 0.7057          & 0.6435          & 0.6962          & 0.8027          & 0.8132          & 0.7544          & 0.6593          & 0.7828          & 0.6750          & 0.7542          \\
            Star          & 0.7202          & 0.6980          & 0.6008          & 0.6974          & 0.7937          & 0.7942          & 0.7759          & 0.6280          & 0.8024          & 0.6578          & 0.7541          \\
            MLP+DN        & 0.7204          & 0.7084          & 0.6363          & 0.6887          & 0.7851          & 0.8107          & 0.7488          & 0.6530          & 0.7694          & 0.6792          & 0.7239          \\
            MLP+DR        & 0.7407          & 0.7248          & 0.6353          & 0.7132          & 0.8167          & 0.8224          & 0.7486          & 0.6761          & 0.8263          & 0.6730          & 0.7681          \\
            MLP+MAMDR     & \textbf{0.7445} & 0.7210          & 0.6541          & \textbf{0.7180} & \textbf{0.8179} & \textbf{0.8242} & 0.7462          & 0.6790          & 0.8242          & \textbf{0.6838} & \textbf{0.7795} \\ \bottomrule
        \end{tabular}%
    }
\end{table}
\begin{table}[h]
    \caption{Results of each domain on Taobao-20 dataset.}
    \label{tab:taobao-20-specific}
    \resizebox{\textwidth}{!}{%
        \begin{tabular}{@{}cccccccccccccccccccccc@{}}
            \toprule
            \textbf{Method} & \textbf{Avg.}   & \textbf{1}      & \textbf{2}      & \textbf{3}      & \textbf{4}      & \textbf{5}      & \textbf{6}      & \textbf{7}      & \textbf{8}      & \textbf{9}      & \textbf{10}     & \textbf{11}     & \textbf{12}     & \textbf{13}     & \textbf{14}     & \textbf{15}     & \textbf{16}     & \textbf{17}     & \textbf{18}     & \textbf{19}     & \textbf{20}     \\ \midrule
            MLP             & 0.7255          & 0.7062          & 0.6002          & 0.6900          & 0.7733          & 0.8060          & 0.7591          & 0.6005          & 0.7638          & 0.6441          & 0.7106          & 0.8516          & 0.7879          & 0.7840          & 0.7860          & 0.7973          & 0.6858          & 0.6864          & 0.7103          & 0.7249          & 0.6426          \\
            WDL             & 0.7235          & 0.7035          & 0.6121          & 0.6857          & 0.7591          & 0.7940          & 0.7575          & 0.6418          & 0.7603          & 0.6593          & 0.7026          & 0.8525          & 0.7939          & 0.7781          & 0.7754          & 0.7964          & 0.6792          & 0.6720          & 0.7151          & 0.7210          & 0.6100          \\
            NFM             & 0.7461          & \textbf{0.7262} & 0.6366          & 0.6900          & 0.7561          & 0.8012          & 0.7576          & 0.6828          & 0.8074          & 0.6863          & 0.7267          & 0.8337          & 0.8007          & 0.8109          & 0.8056          & 0.7986          & 0.6911          & 0.7020          & 0.7560          & 0.7540          & 0.6988          \\
            AutoInt         & 0.7471          & 0.7217          & 0.6192          & 0.6824          & 0.7908          & 0.8150          & \textbf{0.7753} & 0.6268          & 0.8263          & 0.6682          & 0.7483          & 0.8639          & \textbf{0.8127} & \textbf{0.8130} & 0.8165          & 0.8270          & 0.6937          & 0.6890          & 0.7640          & 0.7455          & 0.6428          \\
            DeepFM          & 0.7347          & 0.7052          & 0.6177          & 0.6541          & 0.7553          & 0.7996          & 0.7482          & 0.6395          & 0.8227          & 0.6527          & 0.7052          & 0.8365          & 0.7922          & 0.7985          & 0.8097          & 0.8016          & \textbf{0.7075} & 0.6719          & 0.7192          & 0.7442          & \textbf{0.7130} \\
            Shared-bottom   & 0.7572          & 0.7313          & 0.6348          & 0.7164          & 0.8114          & 0.8216          & 0.7803          & 0.6748          & 0.8078          & \textbf{0.6915} & 0.7719          & 0.8783          & 0.7943          & 0.8183          & 0.8341          & 0.8354          & 0.6879          & 0.7003          & 0.7813          & 0.7338          & 0.6392          \\
            MMOE            & 0.7494          & 0.7135          & 0.6226          & 0.7063          & 0.8060          & 0.8219          & 0.7716          & 0.6568          & 0.7884          & 0.6828          & 0.7535          & 0.8700          & 0.7961          & 0.8125          & 0.8340          & 0.8351          & 0.6911          & 0.6936          & 0.7614          & 0.7249          & 0.6463          \\
            PLE             & 0.7603          & 0.7226          & 0.6412          & 0.7172          & 0.8135          & 0.8290          & 0.7824          & 0.6680          & 0.8124          & 0.6906          & 0.7763          & 0.8784          & 0.7964          & 0.8167          & 0.8414          & 0.8394          & 0.6856          & 0.7040          & 0.7888          & 0.7351          & 0.6661          \\
            Star            & 0.7324          & 0.6901          & 0.5746          & 0.7080          & 0.7956          & 0.7878          & 0.7466          & 0.6371          & 0.7793          & 0.6614          & 0.7588          & 0.8592          & 0.8028          & 0.7872          & 0.8274          & 0.8033          & 0.6218          & 0.6865          & 0.7687          & 0.7185          & 0.6330          \\
            MLP+DN          & 0.7501          & 0.7203          & 0.6264          & 0.6998          & 0.7942          & 0.8209          & 0.7698          & 0.6794          & 0.7943          & 0.6853          & 0.7520          & 0.8678          & 0.7920          & 0.8104          & 0.8195          & 0.8346          & 0.6798          & 0.7001          & 0.7565          & 0.7373          & 0.6617          \\
            MLP+DR          & 0.7596          & 0.7210          & 0.6400          & \textbf{0.7324} & 0.8084          & \textbf{0.8343} & 0.7697          & 0.6714          & 0.8298          & 0.6787          & 0.7776          & 0.8698          & 0.8056          & 0.8015          & 0.8260          & 0.8442          & 0.6583          & 0.7090          & 0.7872          & 0.7506          & 0.6769          \\
            MLP+MAMDR       & \textbf{0.7613} & 0.7162          & \textbf{0.6446} & 0.7306          & \textbf{0.8144} & 0.8315          & 0.7576          & \textbf{0.7085} & \textbf{0.8292} & 0.6782          & \textbf{0.7831} & \textbf{0.8784} & 0.8076          & 0.8015          & \textbf{0.8359} & \textbf{0.8427} & 0.6518          & \textbf{0.7117} & \textbf{0.7914} & \textbf{0.7488} & 0.6628          \\ \bottomrule
        \end{tabular}%
    }
\end{table}
\begin{table}[h]
    \caption{Results of each domain on Taobao-30 dataset.}
    \label{tab:taobao-30-specific}
    \resizebox{\textwidth}{!}{%
        \begin{tabular}{@{}cccccccccccccccccccccccccccccccc@{}}
            \toprule
            Method        & Avg.            & 1               & 2               & 3               & 4               & 5               & 6               & 7               & 8               & 9               & 10              & 11              & 12              & 13              & 14              & 15              & 16              & 17              & 18              & 19              & 20              & 21              & 22              & 23              & 24              & 25              & 26              & 27              & 28              & 29              & 30              \\ \midrule
            MLP           & 0.7416          & 0.7307          & 0.6127          & 0.6979          & 0.7774          & 0.8113          & 0.7601          & 0.6518          & 0.7765          & 0.6742          & 0.7366          & 0.8568          & 0.8004          & 0.7789          & 0.8116          & 0.8311          & 0.6726          & 0.6869          & 0.7332          & 0.7133          & 0.6569          & 0.7629          & 0.7305          & 0.7478          & 0.7390          & 0.6966          & 0.7305          & 0.7576          & 0.8014          & 0.8005          & 0.7086          \\
            WDL           & 0.7559          & 0.7377          & 0.6338          & 0.7019          & 0.7876          & 0.8181          & 0.7722          & 0.6703          & 0.8002          & 0.6697          & 0.7498          & 0.8664          & 0.7999          & 0.7950          & 0.8173          & 0.8446          & 0.6890          & 0.6912          & 0.7579          & 0.7258          & 0.7131          & 0.7717          & 0.7579          & 0.7543          & 0.7536          & 0.7124          & 0.7589          & 0.7665          & 0.8186          & 0.8185          & 0.7233          \\
            NFM           & 0.7673          & 0.7267          & \textbf{0.6591} & 0.6905          & 0.7828          & 0.8065          & 0.7633          & 0.6671          & 0.8294          & 0.6955          & 0.7642          & 0.8550          & 0.8196          & \textbf{0.8067} & 0.8233          & 0.8380          & 0.7241          & 0.7046          & 0.7667          & 0.7331          & \textbf{0.7570} & 0.7858          & 0.7918          & 0.7501          & 0.7601          & 0.7386          & \textbf{0.8282} & 0.7550          & 0.8218          & 0.8254          & 0.7329          \\
            AutoInt       & 0.7623          & 0.7407          & 0.6420          & 0.6972          & 0.7826          & 0.8127          & 0.7773          & 0.6874          & 0.8306          & 0.6528          & 0.7592          & 0.8568          & \textbf{0.8183} & 0.8010          & 0.8107          & 0.8435          & \textbf{0.7196} & 0.7056          & 0.7671          & 0.7400          & 0.6983          & 0.7853          & 0.7828          & 0.7516          & 0.7604          & 0.7292          & 0.7619          & 0.7689          & 0.8246          & 0.8190          & \textbf{0.7409} \\
            DeepFM        & 0.7484          & 0.7224          & 0.6272          & 0.6691          & 0.7672          & 0.8009          & 0.7426          & 0.6475          & 0.8212          & 0.6782          & 0.7271          & 0.8496          & 0.7870          & 0.8066          & 0.8118          & 0.8066          & 0.7231          & 0.6846          & 0.7295          & 0.7366          & 0.7222          & 0.7521          & 0.7736          & 0.7237          & 0.7578          & 0.7099          & 0.8203          & 0.7166          & 0.8030          & 0.8004          & 0.7343          \\
            Shared-bottom & 0.7714          & \textbf{0.7504} & 0.6467          & 0.7087          & 0.8068          & 0.8216          & 0.7812          & 0.6776          & 0.8118          & 0.6878          & 0.7691          & 0.8741          & 0.8007          & 0.8187          & 0.8323          & 0.8467          & 0.6846          & 0.7013          & 0.7793          & 0.7237          & 0.6861          & 0.7769          & 0.7732          & 0.7786          & 0.7587          & 0.7318          & 0.7585          & 0.7765          & 0.8295          & 0.8204          & 0.7255          \\
            MMOE          & 0.7717          & 0.7391          & 0.6453          & 0.7216          & 0.8135          & \textbf{0.8264} & 0.7855          & 0.6691          & 0.8270          & 0.6924          & 0.7810          & \textbf{0.8798} & 0.8007          & 0.8057          & \textbf{0.8410} & 0.8523          & 0.6760          & 0.7115          & 0.7883          & 0.7386          & 0.6794          & 0.7856          & \textbf{0.7975} & 0.7870          & 0.7590          & 0.7420          & 0.7844          & 0.7860          & \textbf{0.8421} & 0.8309          & 0.7307          \\
            PLE           & 0.7725          & 0.7368          & 0.6459          & 0.7157          & 0.8134          & 0.8270          & \textbf{0.7917} & 0.6898          & 0.8265          & \textbf{0.6951} & 0.7809          & 0.8781          & 0.7992          & 0.8080          & 0.8393          & 0.8411          & 0.6998          & 0.7105          & 0.7902          & 0.7440          & 0.7117          & 0.7841          & 0.7896          & 0.7875          & 0.7601          & 0.7459          & 0.7682          & 0.7850          & 0.8381          & 0.8267          & 0.7306          \\
            Star          & 0.7483          & 0.6807          & 0.6323          & 0.7017          & 0.7879          & 0.8011          & 0.7725          & 0.6490          & 0.8065          & 0.6737          & 0.7302          & 0.8628          & 0.8024          & 0.7908          & 0.8179          & 0.8267          & 0.6643          & 0.6883          & 0.7738          & 0.7151          & 0.6542          & 0.7705          & 0.7674          & 0.7601          & 0.7579          & 0.7410          & 0.7458          & 0.7760          & 0.8140          & 0.7859          & 0.6978          \\
            MLP+DN        & 0.7619          & 0.7394          & 0.6474          & 0.7003          & 0.7931          & 0.8222          & 0.7777          & 0.6929          & 0.8118          & 0.6895          & 0.7545          & 0.8686          & 0.8094          & 0.8072          & 0.8231          & 0.8467          & 0.6807          & 0.6992          & 0.7554          & 0.7334          & 0.7084          & 0.7815          & 0.7619          & 0.7660          & 0.7593          & 0.7230          & 0.7594          & 0.7727          & 0.8215          & 0.8215          & 0.7302          \\
            MLP+DR        & 0.7726          & 0.7253          & 0.6640          & 0.7274          & 0.8119          & 0.8274          & 0.7680          & 0.7083          & 0.8359          & 0.6764          & 0.7754          & 0.8744          & 0.8099          & 0.8022          & 0.8285          & 0.8553          & 0.6693          & 0.7125          & 0.7900          & 0.7555          & 0.7066          & 0.7865          & 0.7786          & 0.7856          & 0.7611          & 0.7464          & 0.7931          & 0.7912          & 0.8379          & 0.8331          & 0.7404          \\
            MLP+MAMDR     & \textbf{0.7750} & 0.7357          & 0.6541          & \textbf{0.7296} & \textbf{0.8179} & 0.8243          & 0.7694          & \textbf{0.7111} & \textbf{0.8397} & 0.6764          & \textbf{0.7884} & 0.8760          & 0.8121          & 0.8032          & 0.8360          & \textbf{0.8568} & 0.6806          & \textbf{0.7117} & \textbf{0.7906} & \textbf{0.7644} & 0.6977          & \textbf{0.7919} & 0.7936          & \textbf{0.7901} & \textbf{0.7641} & \textbf{0.7482} & 0.7878          & \textbf{0.7941} & 0.8371          & \textbf{0.8324} & 0.7338          \\ \bottomrule
        \end{tabular}%
    }
\end{table}
